# Supplementary material for: Architectural mechanisms of a universal fault-tolerant quantum computer
Source: arXiv:2506.20661 ancillary file (2025-06-25)
Supplement: Supplementary file 1 [file RawExperimentalCommands_SurfaceCodeQEC.pdf]

## Moving AWG command string

The command string used to program the RF waveforms for the Moving AWG, which control the positions and powers of moveable AOD tweezers, is given below. Waveforms are uploaded to different segments of the AWG using the SEGMENT[] command, which can then be individually looped or triggered with an external trigger.

Each move is defined using a MOVEAOD command. The initial position and power is specified for the first command when tweezers are turned on. For subsequent commands, the arguments specify where to move to (and optionally the power to ramp to), and take the form MOVEAOD[[x\_positions, y\_positions],[xpowers,ypowers],) time\_for\_move]. Additional arguments such as SHIFT apply a global (x,y) coordinate shift to the coordinates in that move. Coordinates are given in 'SLM units' where 1 SLM unit here is approximately 4.6um in the x direction and 4.9um in the y direction (corresponding to 7 and 7.5 units in the corresponding Supplementary Video, respectively)

### Define coordinates and powers

```
COMB[xd_ent, [13,3,6]]
COMB[yd_ent, [2,2,6]]
COMB[ykill_ent, [0, 2, 7]]
REPEAT_VAL[xkill_pow, [0.4, 6]]
REPEAT_VAL[ykill_pow, [1.65, 7]]
```

```
COMB[xanc_ent, [14.86,3,6]]
COMB[yanc_ent, [1,2,6]]
```

```
REPEAT_VAL[xno6_pow, [0.14, 6]]
REPEAT_VAL[yno6_pow, [0.0001, 6]]
REPEAT_VAL[yno7_pow, [0.0001, 7]]
```

```
REPEAT_VAL[xpow_imaging, [0.25, 6]]
REPEAT_VAL[ypow_imaging, [1.01, 6]]
```

```
REPEAT_VAL[xpow_gates, [0.18, 6]]
REPEAT_VAL[ypow_gates, [0.91, 6]]
```

```
COMB[x_st, [-0.98, 3, 6]]
COMB[y_st, [21, 1.98, 6]]
```

```
REPEAT_VAL[xpow_pickup, [0.36, 6]]
REPEAT_VAL[ypow_pickup, [1.83, 6]]
REPEAT_VAL[x2pow_pickup, [0.36, 6]]
REPEAT_VAL[y2pow_pickup, [1.33, 6]]
```

```
COMB[x_ssr, [-0.98,2,18]]
```

```
VAR[xpow1_ssr,
[0.26,0.26,0.24,0.24,0.22,0.21,0.21,0.21,0.21,0.21,0.21,0.23,0.23,0.23,0.24,0.24,0.24,0.20]]
REPEAT_VAL[xno18_pow, [0.0001,18]]
VAR[y3pow_pickup, [1.19, 1.20, 1.23, 1.28, 1.29, 1.47]]
```

### First segment, used to clear unwanted atoms from entangling zone traps

```

SEGMENT[1, LOOP_UNTIL_TRIG]
MoveAOD[Initial[xd_ent, ykill_ent],
InitialPows[xkill_pow, yno7_pow],
FinalPows[xkill_pow,ykill_pow], 0.1 ms]
MoveAOD[[xd_ent, ykill_ent], SHIFT[[-1.5],[-1]], 0.1 ms]
WAIT[0.02 ms]

```

### Second segment, move atoms to their positions for the start of the circuit

```

SEGMENT[2]
MoveAOD[Initial[x_st, y_st],
InitialPows[xno6_pow, xno6_pow],
FinalPows[xpow_pickup,ypow_pickup],0.2 ms]
SAVE_PREVIOUS[]

NOTE[Move data qubits to the entangling zone]
MoveAOD[[x_st,y_st],SHIFT[[0.5],[0]],0.1 ms]
MoveAOD[[x_st,yd_ent],SHIFT[[0.5],[-0.5]],0.4 ms]
MoveAOD[[xd_ent,yd_ent],SHIFT[[0],[-0.5]],0.2 ms]
MoveAOD[[xd_ent,yd_ent],SHIFT[[0],[0]],0.1 ms]
MoveAOD[[xd_ent,yd_ent],FinalPows[xno6_pow,xno6_pow],0.3 ms]

```

```

NOTE[Move first ancilla set to entangling zone]
MoveAOD[Initial[x_st,y_st],SHIFT[[1],[0]],
InitialPows[xno6_pow, xno6_pow],
FinalPows[xpow_pickup, ypow_pickup],0.2 ms]

MoveAOD[[x_st,y_st],SHIFT[[1.5],[0]],0.1 ms]
MoveAOD[[x_st,yanc_ent],SHIFT[[1.5],[0]],0.3 ms]
MoveAOD[[xanc_ent,yanc_ent], 0.3 ms]
MoveAOD[[xanc_ent,yanc_ent], FinalPows[xpow_imaging, ypow_imaging],0.05ms]
SAVE_PREVIOUS[]
SAVE_PREVIOUS[]

```

### Start of circuit

```

SEGMENT[4]

Wait[1 us]
MoveAOD[[xanc_ent,yanc_ent], FinalPows[xpow_gates, ypow_gates], 0.1 ms]

NOTE[Data pi/2 pulses for first round]
Wait[403 us]
NOTE[Fake ancilla pi/2 pulses, first round]
Wait[70 us]
NOTE[Data qubit pi pulse, followed by Ancilla pi/2 pulses]

Wait[70 us]
MoveAOD[[xanc_ent,yanc_ent], SHIFT[[-1.5],[1]], 0.195 ms]
Wait[10 us]
MoveAOD[[xanc_ent,yanc_ent], SHIFT[[0],[0]], 0.195 ms]
Wait[70 us]
MoveAOD[[xanc_ent,yanc_ent], SHIFT[[-1.5],[-1]], 0.195 ms]

```

```
Wait[10 us]
MoveAOD[[xanc_ent,yanc_ent], SHIFT[[0],[0]], 0.195 ms]
Wait[70 us]
MoveAOD[[xanc_ent,yanc_ent], SHIFT[[0.75],[1]], 0.195 ms]
Wait[10 us]
MoveAOD[[xanc_ent,yanc_ent], SHIFT[[0],[0]], 0.195 ms]
Wait[70 us]
MoveAOD[[xanc_ent,yanc_ent], SHIFT[[0.78],[-1]], 0.195 ms]
Wait[10 us]
MoveAOD[[xanc_ent,yanc_ent], SHIFT[[0],[0]], 0.195 ms]
Wait[70 us]
```

NOTE[Move back to original spot]

```
MoveAOD[[xanc_ent,yanc_ent], FinalPows[x2pow_pickup, y2pow_pickup], 0.1 ms]
MoveAOD[[x_st,yanc_ent],SHIFT[[1.53],[0]],0.4 ms]
MoveAOD[[x_st,y_st],SHIFT[[1.53],[0]],0.4 ms]
MoveAOD[[x_st,y_st], SHIFT[[1.03],[0]],0.1 ms]
MoveAOD[[x_st,y_st], FinalPows[xno6_pow, yno6_pow], SHIFT[[1.03],[0]], 0.250 ms]
```

NOTE[Pick up next group of atoms, and do again. Exchanging the ancilla arrays is currently given 1 ms total time.]

```
MoveAOD[Initial[x_st,y_st], InitialPows[xno6_pow, yno6_pow],
FinalPows[x2pow_pickup, y2pow_pickup],SHIFT[[1.938],[0]], 0.250 ms]
MoveAOD[[x_st,y_st],SHIFT[[2.438],[0]],0.1 ms]
MoveAOD[[x_st,yanc_ent],SHIFT[[2.438],[0]],0.4 ms]
MoveAOD[[xanc_ent,yanc_ent], 0.4 ms]
MoveAOD[[xanc_ent,yanc_ent], SHIFT[[0],[0]], FinalPows[xpow_gates, ypow_gates],
0.1 ms]
```

```
Wait[70 us]
MoveAOD[[xanc_ent,yanc_ent], SHIFT[[-1.5],[1]], 0.195 ms]
Wait[10 us]
MoveAOD[[xanc_ent,yanc_ent], SHIFT[[0],[0]], 0.195 ms]
Wait[70 us]
MoveAOD[[xanc_ent,yanc_ent], SHIFT[[0.78],[1]], 0.195 ms]
Wait[10 us]
MoveAOD[[xanc_ent,yanc_ent], SHIFT[[0],[0]], 0.195 ms]
Wait[70 us]
MoveAOD[[xanc_ent,yanc_ent], SHIFT[[-1.5],[-1]], 0.195 ms]
Wait[10 us]
MoveAOD[[xanc_ent,yanc_ent], SHIFT[[0],[0]], 0.195 ms]
Wait[70 us]
MoveAOD[[xanc_ent,yanc_ent], SHIFT[[0.78],[-1]], 0.195 ms]
Wait[10 us]
MoveAOD[[xanc_ent,yanc_ent], SHIFT[[0],[0]], 0.195 ms]
Wait[70 us]
```

```
MoveAOD[[xanc_ent,yanc_ent], FinalPows[x2pow_pickup, y2pow_pickup], 0.1 ms]
MoveAOD[[x_st,yanc_ent],SHIFT[[2.438],[0]],0.4 ms]
MoveAOD[[x_st,y_st],SHIFT[[2.438],[0]],0.4 ms]
MoveAOD[[x_st,y_st], SHIFT[[1.938],[0]],0.1 ms]
```

MoveAOD[[x\_st,y\_st], FinalPows[xno6\_pow, yno6\_pow], SHIFT[[1.938],[0]], 0.250 ms]

Note[Third ancilla block]

MoveAOD[Initial[x\_st,y\_st], InitialPows[xno6\_pow, yno6\_pow],  
FinalPows[x2pow\_pickup, y2pow\_pickup],SHIFT[[17.959],[0]], 0.250 ms]  
MoveAOD[[x\_st,y\_st],SHIFT[[18.459],[0]],0.1 ms]  
MoveAOD[[x\_st,yanc\_ent],SHIFT[[18.459],[0]],0.4 ms]  
MoveAOD[[xanc\_ent,yanc\_ent], 0.4 ms]  
MoveAOD[[xanc\_ent,yanc\_ent], SHIFT[[0],[0]], FinalPows[xpow\_gates, ypow\_gates],  
0.1 ms]

Wait[70 us]  
MoveAOD[[xanc\_ent,yanc\_ent], SHIFT[[0.78],[-1]], 0.195 ms]  
Wait[10 us]  
MoveAOD[[xanc\_ent,yanc\_ent], SHIFT[[0],[0]], 0.195 ms]  
Wait[70 us]  
MoveAOD[[xanc\_ent,yanc\_ent], SHIFT[[-1.5],[-1]], 0.195 ms]  
Wait[10 us]  
MoveAOD[[xanc\_ent,yanc\_ent], SHIFT[[0],[0]], 0.195 ms]  
Wait[70 us]  
MoveAOD[[xanc\_ent,yanc\_ent], SHIFT[[0.78],[1]], 0.195 ms]  
Wait[10 us]  
MoveAOD[[xanc\_ent,yanc\_ent], SHIFT[[0],[0]], 0.195 ms]  
Wait[70 us]  
MoveAOD[[xanc\_ent,yanc\_ent], SHIFT[[-1.5],[1]], 0.195 ms]  
Wait[10 us]  
MoveAOD[[xanc\_ent,yanc\_ent], SHIFT[[0],[0]], 0.195 ms]  
Wait[70 us]

MoveAOD[[xanc\_ent,yanc\_ent], FinalPows[x2pow\_pickup, y2pow\_pickup], 0.1 ms]  
MoveAOD[[x\_st,yanc\_ent],SHIFT[[18.459],[0]],0.4 ms]  
MoveAOD[[x\_st,y\_st],SHIFT[[18.459],[0]],0.4 ms]  
MoveAOD[[x\_st,y\_st], SHIFT[[17.959],[0]],0.1 ms]  
MoveAOD[[x\_st,y\_st], FinalPows[xno6\_pow, yno6\_pow], SHIFT[[17.959],[0]], 0.250 ms]

Note[Fourth ancilla block]

MoveAOD[Initial[x\_st,y\_st], InitialPows[xno6\_pow, yno6\_pow],  
FinalPows[x2pow\_pickup, y2pow\_pickup],SHIFT[[18.972],[0]], 0.250 ms]  
MoveAOD[[x\_st,y\_st],SHIFT[[19.472],[0]],0.1 ms]  
MoveAOD[[x\_st,yanc\_ent],SHIFT[[19.472],[0]],0.4 ms]  
MoveAOD[[xanc\_ent,yanc\_ent], 0.4 ms]  
MoveAOD[[xanc\_ent,yanc\_ent], SHIFT[[0],[0]], FinalPows[xpow\_gates, ypow\_gates],  
0.1 ms]

Wait[70 us]  
MoveAOD[[xanc\_ent,yanc\_ent], SHIFT[[0.78],[-1]], 0.195 ms]  
Wait[10 us]  
MoveAOD[[xanc\_ent,yanc\_ent], SHIFT[[0],[0]], 0.195 ms]  
Wait[70 us]  
MoveAOD[[xanc\_ent,yanc\_ent], SHIFT[[0.78],[1]], 0.195 ms]

```

Wait[10 us]
MoveAOD[[xanc_ent,yanc_ent], SHIFT[[0],[0]], 0.195 ms]
Wait[70 us]
MoveAOD[[xanc_ent,yanc_ent], SHIFT[[-1.5],[-1]], 0.195 ms]
Wait[10 us]
MoveAOD[[xanc_ent,yanc_ent], SHIFT[[0],[0]], 0.195 ms]
Wait[70 us]
MoveAOD[[xanc_ent,yanc_ent], SHIFT[[-1.5],[1]], 0.195 ms]
Wait[10 us]
MoveAOD[[xanc_ent,yanc_ent], SHIFT[[0],[0]], 0.195 ms]
Wait[70 us]

MoveAOD[[xanc_ent,yanc_ent], FinalPows[x2pow_pickup, y2pow_pickup], 0.1 ms]
MoveAOD[[x_st,yanc_ent],SHIFT[[19.472],[0]],0.4 ms]
MoveAOD[[x_st,y_st],SHIFT[[19.472],[0]],0.4 ms]
MoveAOD[[x_st,y_st], SHIFT[[18.972],[0]],0.1 ms]
MoveAOD[[x_st,y_st], FinalPows[xno6_pow, yno6_pow], SHIFT[[18.972],[0]], 0.250
ms]

Note[Move data back to storage zone, 1.2 ms]

MoveAOD[Initial[xd_ent, yd_ent], InitialPows[xno6_pow, yno6_pow],
FinalPows[x2pow_pickup,y2pow_pickup], 0.35 ms]
MoveAOD[[xd_ent,yd_ent],SHIFT[[0],[-0.5]],0.2 ms]
MoveAOD[[x_st,yd_ent], SHIFT[[0.53],[-0.5]],0.3 ms]
MoveAOD[[x_st,y_st], SHIFT[[0.53],[0]],0.5 ms]
MoveAOD[[x_st,y_st], SHIFT[[0.03],[0]],0.2 ms]
MoveAOD[[x_st,y_st], FinalPows[xno6_pow, yno6_pow], SHIFT[[0.03],[0]], 0.3 ms]

SEGMENT[6]
Note[SSR on half, 1.2 ms]

WAIT[0.2 ms]

MoveAOD[Initial[x_ssr, y_st],
InitialPows[xno18_pow, yno6_pow],
FinalPows[xpow1_ssr,y3pow_pickup],0.5 ms]
WAIT[100 us]
MoveAOD[[x_ssr, y_st], SHIFT[[0.5],[0]], 0.7 ms]
MoveAOD[[x_ssr, y_st], SHIFT[[0.5],[-1]],0.2 ms]
MoveAOD[[x_ssr, y_st], SHIFT[[0],[-1]],0.1 ms]
MoveAOD[[x_ssr,y_st], FinalPows[xno18_pow, yno6_pow], SHIFT[[0],[-1]], 0.3 ms]

Note[SSR on half, 1.23 ms]

MoveAOD[Initial[x_ssr, y_st],
InitialPows[xno18_pow, yno6_pow],
FinalPows[xpow1_ssr,y3pow_pickup], SHIFT[[1],[0]],0.5 ms]
WAIT[100 us]
MoveAOD[[x_ssr, y_st], SHIFT[[1.5],[0]], 0.7 ms]
MoveAOD[[x_ssr, y_st], SHIFT[[1.5],[-1]],0.2 ms]
MoveAOD[[x_ssr, y_st], SHIFT[[1],[-1]],0.1 ms]
MoveAOD[[x_ssr,y_st], FinalPows[xno18_pow, yno6_pow], SHIFT[[1],[-1]], 0.3 ms]

```

END\_COMMAND[ ]

## Raman AWG command string

The command string used to program the I/Q waveforms and AOM amplitudes for local and global Raman control is given below. The command specifies the parameters for each single-qubit gate, which is then converted into the appropriate waveforms to modulate the light intensity and microwave phase and frequency (defined relative to the resonance frequency).

For local gates, the pulses are optionally gated on and off by the Raman AOD command.

Examples of typical commands are

Z : global Z rotation, in units of  $2\pi$

E : wait time, idling at the specified frequency

SC1\_ECHO : global SCROFULOUS  $Y(\pi)$  pulse for dynamical decoupling, idling at the specified frequency

SC1\_H\_FIXEDLOOPED\_SMOOTH\_PCOMP : SCROFULOUS  $Y(\pi/2)$  local gaussian pulses

SC1PI\_FIXEDLOOPED\_SMOOTH\_PCOMP : SCROFULOUS  $Y(\pi)$  local gaussian pulses

BB1\_FIXED: global BB1 pulse

### State preparation before circuit begins

E[50.5 us, 12 MHz]

CPROBUST180\_OFFSETFREQSMOOTH\_COMPENSATED[1.73 us, 0.035 us, 12.1056 MHz, 0.75, 4]

E[0.2 us, 8.3 MHz]

CPROBUST180\_OFFSETFREQSMOOTH[2.455 us, 0.035 us, 4.063 MHz, 1, 4]

E[2.65 us, 0.1 MHz]

SEGMENTBREAK[1896]

E[16.6 us, 0.1 MHz]

BB1\_FIXED[0.5,0.12 us,5.65 us]

E[4 us, 5 MHz]

SMOOTHPUMPINGLOOPEDTTL[0, 2.18 us, -11.7 MHz, 11.7 MHz, 1, 4, 24, 8.53 us, 0.1us, 3us]

E[494.052 us, 5 MHz]

### Start of circuit

# Prepare data qubit

SC1\_ECHO[6 us, 0 MHz]

SC1\_H\_FIXEDLOOPED\_SMOOTH\_PCOMP[0.01us, 0.88, 4, 5.8180 us, 0.46744, 3, local]

SC1PI\_FIXEDLOOPED\_SMOOTH\_PCOMP[0.01us, 0.88, 4, 5.8180 us, 0.45710, 6, local]

Z[0.45710]

SC1\_H\_FIXEDLOOPED\_SMOOTH\_PCOMP[0.01us, 0.88, 4, 5.8180 us, 0.46744, 3, local]

# Start first QEC round

Z[0]

E[397.968 us, 0.07 MHz]

Z[0.000]

SC1\_H\_FIXEDLOOPED\_SMOOTH\_PCOMP[0.01us, 0.88, 4, 5.8180 us, 0.46744, 6, local]

SC1\_ECHO[76 us, 0.07 MHz]

SC1\_H\_FIXEDLOOPED\_SMOOTH\_PCOMP[0.01us, 0.88, 4, 5.8180 us, 0.46744, 6, local]

Z[0.287]

E[397.968 us, 0.07 MHz]  
Z[0.000]

SC1\_H\_FIXEDLOOPED\_SMOOTH\_PCOMP[0.01us, 0.88, 4, 5.8180 us, 0.46744, 3, local]  
Z[0.46744]  
SC1PI\_FIXEDLOOPED\_SMOOTH\_PCOMP[0.01us, 0.88, 4, 5.8180 us, 0.45710, 6, local]  
SC1\_H\_FIXEDLOOPED\_SMOOTH\_PCOMP[0.01us, 0.88, 4, 5.8180 us, 0.46744, 3, local]  
Z[0.46744]

Z[0.000]  
Z[0.287]  
E[397.968 us, 0.07 MHz]  
SC1\_H\_FIXEDLOOPED\_SMOOTH\_PCOMP[0.01us, 0.88, 4, 5.8180 us, 0.46744, 6, local]  
SC1\_ECHO[4 us, 0.07 MHz]  
SC1\_H\_FIXEDLOOPED\_SMOOTH\_PCOMP[0.01us, 0.88, 4, 5.8180 us, 0.46744, 6, local]  
E[397.968 us, 0.07 MHz]  
Z[0.287]  
Z[0.000]

Z[0.46744]  
SC1\_H\_FIXEDLOOPED\_SMOOTH\_PCOMP[0.01us, 0.88, 4, 5.8180 us, 0.46744, 3, local]  
SC1PI\_FIXEDLOOPED\_SMOOTH\_PCOMP[0.01us, 0.88, 4, 5.8180 us, 0.45710, 6, local]  
Z[0.46744]  
SC1\_H\_FIXEDLOOPED\_SMOOTH\_PCOMP[0.01us, 0.88, 4, 5.8180 us, 0.46744, 3, local]

Z[0.287]  
E[397.968 us, 0.07 MHz]  
Z[0.000]

SC1\_H\_FIXEDLOOPED\_SMOOTH\_PCOMP[0.01us, 0.88, 4, 5.8180 us, 0.46744, 6, local]

Z[0.000]  
SC1\_ECHO[2574.028 us, 0.07 MHz]  
Z[0.000]

# Start second QEC round

SC1\_H\_FIXEDLOOPED\_SMOOTH\_PCOMP[0.01us, 0.88, 4, 5.8180 us, 0.46744, 6, local]

Z[0.287]  
E[397.968 us, 0.07 MHz]  
Z[0.000]

SC1\_H\_FIXEDLOOPED\_SMOOTH\_PCOMP[0.01us, 0.88, 4, 5.8180 us, 0.46744, 3, local]  
Z[0.46744]  
SC1PI\_FIXEDLOOPED\_SMOOTH\_PCOMP[0.01us, 0.88, 4, 5.8180 us, 0.45710, 6, local]  
SC1\_H\_FIXEDLOOPED\_SMOOTH\_PCOMP[0.01us, 0.88, 4, 5.8180 us, 0.46744, 3, local]  
Z[0.46744]

Z[0.000]  
Z[0.287]  
E[397.968 us, 0.07 MHz]  
SC1\_H\_FIXEDLOOPED\_SMOOTH\_PCOMP[0.01us, 0.88, 4, 5.8180 us, 0.46744, 6, local]  
SC1\_ECHO[4 us, 0.07 MHz]



SC1\_H\_FIXEDLOOPED\_SMOOTH\_PCOMP[0.01us, 0.88, 4, 5.8180 us, 0.46744, 6, local]  
E[397.968 us, 0.07 MHz]  
Z[0.287]  
Z[0.000]

Z[0.46744]  
SC1\_H\_FIXEDLOOPED\_SMOOTH\_PCOMP[0.01us, 0.88, 4, 5.8180 us, 0.46744, 3, local]  
SC1PI\_FIXEDLOOPED\_SMOOTH\_PCOMP[0.01us, 0.88, 4, 5.8180 us, 0.45710, 6, local]  
Z[0.46744]  
SC1\_H\_FIXEDLOOPED\_SMOOTH\_PCOMP[0.01us, 0.88, 4, 5.8180 us, 0.46744, 3, local]

Z[0.287]  
E[397.968 us, 0.07 MHz]  
Z[0.000]

SC1\_H\_FIXEDLOOPED\_SMOOTH\_PCOMP[0.01us, 0.88, 4, 5.8180 us, 0.46744, 6, local]  
  
Z[0.000]  
SC1\_ECHO[2574.028 us, 0.07 MHz]  
Z[0.000]

# Start third QEC round

SC1\_H\_FIXEDLOOPED\_SMOOTH\_PCOMP[0.01us, 0.88, 4, 5.8180 us, 0.46744, 6, local]  
  
Z[0.287]  
E[397.968 us, 0.07 MHz]  
Z[0.000]

SC1\_H\_FIXEDLOOPED\_SMOOTH\_PCOMP[0.01us, 0.88, 4, 5.8180 us, 0.46744, 3, local]  
Z[0.46744]  
SC1PI\_FIXEDLOOPED\_SMOOTH\_PCOMP[0.01us, 0.88, 4, 5.8180 us, 0.45710, 6, local]  
SC1\_H\_FIXEDLOOPED\_SMOOTH\_PCOMP[0.01us, 0.88, 4, 5.8180 us, 0.46744, 3, local]  
Z[0.46744]

Z[0.000]  
Z[0.287]  
E[397.968 us, 0.07 MHz]  
SC1\_H\_FIXEDLOOPED\_SMOOTH\_PCOMP[0.01us, 0.88, 4, 5.8180 us, 0.46744, 6, local]  
SC1\_ECHO[4 us, 0.07 MHz]  
SC1\_H\_FIXEDLOOPED\_SMOOTH\_PCOMP[0.01us, 0.88, 4, 5.8180 us, 0.46744, 6, local]  
E[397.968 us, 0.07 MHz]  
Z[0.287]  
Z[0.000]

Z[0.46744]  
SC1\_H\_FIXEDLOOPED\_SMOOTH\_PCOMP[0.01us, 0.88, 4, 5.8180 us, 0.46744, 3, local]  
SC1PI\_FIXEDLOOPED\_SMOOTH\_PCOMP[0.01us, 0.88, 4, 5.8180 us, 0.45710, 6, local]  
Z[0.46744]  
SC1\_H\_FIXEDLOOPED\_SMOOTH\_PCOMP[0.01us, 0.88, 4, 5.8180 us, 0.46744, 3, local]

Z[0.287]

E[397.968 us, 0.07 MHz]  
Z[0.000]

SC1\_H\_FIXEDLOOPED\_SMOOTH\_PCOMP[0.01us, 0.88, 4, 5.8180 us, 0.46744, 6, local]

Z[0.000]  
SC1\_ECHO[2574.028 us, 0.07 MHz]  
Z[0.000]

# Start fourth QEC round

SC1\_H\_FIXEDLOOPED\_SMOOTH\_PCOMP[0.01us, 0.88, 4, 5.8180 us, 0.46744, 6, local]

Z[0.287]  
E[397.968 us, 0.07 MHz]  
Z[0.000]

SC1\_H\_FIXEDLOOPED\_SMOOTH\_PCOMP[0.01us, 0.88, 4, 5.8180 us, 0.46744, 3, local]  
Z[0.46744]  
SC1PI\_FIXEDLOOPED\_SMOOTH\_PCOMP[0.01us, 0.88, 4, 5.8180 us, 0.45710, 6, local]  
SC1\_H\_FIXEDLOOPED\_SMOOTH\_PCOMP[0.01us, 0.88, 4, 5.8180 us, 0.46744, 3, local]  
Z[0.46744]

Z[0.000]  
Z[0.287]  
E[397.968 us, 0.07 MHz]  
SC1\_H\_FIXEDLOOPED\_SMOOTH\_PCOMP[0.01us, 0.88, 4, 5.8180 us, 0.46744, 6, local]  
SC1\_ECHO[4 us, 0.07 MHz]  
SC1\_H\_FIXEDLOOPED\_SMOOTH\_PCOMP[0.01us, 0.88, 4, 5.8180 us, 0.46744, 6, local]  
E[397.968 us, 0.07 MHz]  
Z[0.287]  
Z[0.000]

Z[0.46744]  
SC1\_H\_FIXEDLOOPED\_SMOOTH\_PCOMP[0.01us, 0.88, 4, 5.8180 us, 0.46744, 3, local]  
SC1PI\_FIXEDLOOPED\_SMOOTH\_PCOMP[0.01us, 0.88, 4, 5.8180 us, 0.45710, 6, local]  
Z[0.46744]  
SC1\_H\_FIXEDLOOPED\_SMOOTH\_PCOMP[0.01us, 0.88, 4, 5.8180 us, 0.46744, 3, local]

Z[0.287]  
E[397.968 us, 0.07 MHz]  
Z[0.000]

SC1\_H\_FIXEDLOOPED\_SMOOTH\_PCOMP[0.01us, 0.88, 4, 5.8180 us, 0.46744, 6, local]

SC1\_ECHO[76 us, 0.07 MHz]

SC1\_H\_FIXEDLOOPED\_SMOOTH\_PCOMP[0.01us, 0.88, 4, 5.8180 us, 0.46744, 6, local]  
Z[0]  
E[397.968 us, 0.07 MHz]  
Z[0.000]

# Readout data qubits

SC1\_H\_FIXEDLOOPED\_SMOOTH\_PCOMP[0.01us, 0.88, 4, 5.8180 us, 0.46744, 3, local]

SC1PI\_FIXEDLOOPED\_SMOOTH\_PCOMP[0.01us, 0.88, 4, 5.8180 us, 0.45710, 6, local]  
Z[0.46744]

SC1\_H\_FIXEDLOOPED\_SMOOTH\_PCOMP[0.01us, 0.88, 4, 5.8180 us, 0.46744, 3, local]

# Bright state transfer for spin-to-position conversion

E[2.872 ms, 5 MHz]

BB1\_FIXED[0.5,0.1us,6us]

E[1.819ms, 5MHz]

CPROBUST180\_OFFSETFREQSMOOTH[4.55 us, 0.035 us, 4.083 MHz, 1, 4]

E[0.2 us, 8.3 MHz]

CPROBUST180\_OFFSETFREQSMOOTH\_COMPENSATED[3.1 us, 0.035 us, 12.3256 MHz, 0.75, 4]

END\_COMMAND[ ]

## Raman AOD AWG command string

The command string used to program the RF waveforms for the Raman AOD AWG, which controls the positions and powers of 2D grids of optical tweezers used for local single-qubit gates, is given below.

Positions and powers are separately calibrated and loaded from a saved file. Different pulse configurations are specified by variables, for example in this circuit:

r0\_Ad --> row 0, sublattice A of data qubits  
r0\_a --> row 0, ancilla qubits  
r2\_nl\_a --> row 2, no left edge, ancilla qubits  
r1\_r\_a --> row 1, right edge only, ancilla qubits

```
FILE[repetitiveQEC_d5_variables.txt] # Coordinates are loaded from file
VAR[time[], WAIT[5.8233us]]
VAR[turnoff[], MOVEAOD[Initial[[-3],[-3]],INITIALPOWS[[0],[0]],10ns]]
WAIT[57.47 us]
```

### Start of circuit

# Prepare data qubit in logical state

```
r0_Ad[]
time[]
r1_Ad[]
time[]
r2_Ad[]
time[]
turnoff[]
WAIT[34.99us]
r3_Ad[]
time[]
r4_Ad[]
time[]
r5_Ad[]
time[]
turnoff[]
```

# Start first QEC round

```
WAIT[398.02us]
```

```
WAIT[70us]
WAIT[6us]
WAIT[35us]
r0_a[]
time[]
r1_a[]
time[]
r2_nl_a[]
time[]
r3_a[]
time[]
r4_nl_a[]
```

```
time[]  
r5_a[]  
time[]
```

```
turnoff[]  
WAIT[398.02us]
```

```
r5_d[]  
time[]  
r4_d[]  
time[]  
r3_d[]  
time[]  
turnoff[]  
time[]  
r1_r_a[]  
time[]  
turnoff[]  
time[]  
r3_r_a[]  
time[]  
turnoff[]  
time[]  
turnoff[]  
time[]  
r2_d[]  
time[]  
r1_d[]  
time[]  
r0_d[]  
time[]
```

```
turnoff[]  
WAIT[397.99us]  
turnoff[]  
time[]  
r1_r_a[]  
time[]  
turnoff[]  
time[]  
r3_r_a[]  
time[]  
turnoff[]  
time[]  
turnoff[]  
time[]  
turnoff[]  
WAIT[3.99us]  
turnoff[]  
time[]  
r4_l_a[]  
time[]  
turnoff[]  
time[]
```

```
r2_l_a[]  
time[]  
turnoff[]  
time[]  
turnoff[]  
time[]  
turnoff[]  
WAIT[397.99us]
```

```
r0_d[]  
time[]  
r1_d[]  
time[]  
r2_d[]  
time[]  
turnoff[]  
time[]  
r4_l_a[]  
time[]  
turnoff[]  
time[]  
r2_l_a[]  
time[]  
turnoff[]  
time[]  
turnoff[]  
time[]  
r3_d[]  
time[]  
r4_d[]  
time[]  
r5_d[]  
time[]
```

```
turnoff[]  
WAIT[398.02us]  
r5_a[]  
time[]  
r4_a[]  
time[]  
r3_nr_a[]  
time[]  
r2_a[]  
time[]  
r1_nr_a[]  
time[]  
r0_a[]  
time[]  
turnoff[]  
WAIT[34.99us]
```

```
turnoff[]  
WAIT[2503.99us]
```

```
# Start second QEC round
```

```
WAIT[35us]
```

```
r0_a[]
```

```
time[]
```

```
r1_a[]
```

```
time[]
```

```
r2_a[]
```

```
time[]
```

```
r3_a[]
```

```
time[]
```

```
r4_a[]
```

```
time[]
```

```
turnoff[]
```

```
time[]
```

```
turnoff[]
```

```
WAIT[398.02us]
```

```
r5_d[]
```

```
time[]
```

```
r4_d[]
```

```
time[]
```

```
r3_d[]
```

```
time[]
```

```
r0_a[]
```

```
time[]
```

```
turnoff[]
```

```
time[]
```

```
turnoff[]
```

```
time[]
```

```
turnoff[]
```

```
time[]
```

```
turnoff[]
```

```
time[]
```

```
turnoff[]
```

```
time[]
```

```
r2_d[]
```

```
time[]
```

```
r1_d[]
```

```
time[]
```

```
r0_d[]
```

```
time[]
```

```
turnoff[]
```

```
WAIT[397.99us]
```

```
r0_a[]
```

```
time[]
```

```
turnoff[]
```

```
time[]
```

```
turnoff[]
```

```
time[]
```

```
turnoff[]  
time[]  
turnoff[]  
time[]  
turnoff[]  
time[]  
turnoff[]  
WAIT[3.99us]  
r5_a[]  
time[]  
turnoff[]  
time[]  
turnoff[]  
time[]  
turnoff[]  
time[]  
turnoff[]  
time[]  
turnoff[]  
time[]  
turnoff[]  
WAIT[397.99us]
```

```
r0_d[]  
time[]  
r1_d[]  
time[]  
r2_d[]  
time[]  
r5_a[]  
time[]  
turnoff[]  
time[]  
turnoff[]  
time[]  
turnoff[]  
time[]  
turnoff[]  
time[]  
turnoff[]  
time[]  
r3_d[]  
time[]  
r4_d[]  
time[]  
r5_d[]  
time[]
```

```
turnoff[]  
WAIT[398.02us]  
r5_a[]  
time[]  
r4_a[]  
time[]
```



```
r3_a[]
time[]
r2_a[]
time[]
r1_a[]
time[]
turnoff[]
time[]
turnoff[]
WAIT[34.99us]

turnoff[]
WAIT[2503.99us]
```

```
# Start third QEC round
```

```
WAIT[35us]
turnoff[]
time[]
r1_a[]
time[]
r2_a[]
time[]
r3_a[]
time[]
r4_a[]
time[]
r5_a[]
time[]

turnoff[]
WAIT[398.02us]
```

```
r5_d[]
time[]
r4_d[]
time[]
r3_d[]
time[]
turnoff[]
time[]
turnoff[]
time[]
turnoff[]
time[]
turnoff[]
time[]
turnoff[]
time[]
r5_a[]
time[]
r2_d[]
```

```
time[]
r1_d[]
time[]
r0_d[]
time[]
```

```
turnoff[]
WAIT[397.99us]
turnoff[]
time[]
turnoff[]
time[]
turnoff[]
time[]
turnoff[]
time[]
turnoff[]
time[]
r5_a[]
time[]
turnoff[]
WAIT[3.99us]
turnoff[]
time[]
turnoff[]
time[]
turnoff[]
time[]
turnoff[]
time[]
turnoff[]
time[]
r0_a[]
time[]
turnoff[]
WAIT[397.99us]
```

```

r0_d[]
time[]
r1_d[]
time[]
r2_d[]
time[]
turnoff[]
time[]
turnoff[]
time[]
turnoff[]
time[]
turnoff[]
time[]
turnoff[]
time[]
r0_a[]

```

```
time[]  
r3_d[]  
time[]  
r4_d[]  
time[]  
r5_d[]  
time[]
```

```
turnoff[]  
WAIT[398.02us]  
turnoff[]  
time[]  
r4_a[]  
time[]  
r3_a[]  
time[]  
r2_a[]  
time[]  
r1_a[]  
time[]  
r0_a[]  
time[]  
turnoff[]  
WAIT[34.99us]
```

```
turnoff[]  
WAIT[2503.99us]
```

```
# Start fourth QEC round
```

```
WAIT[35us]  
r0_a[]  
time[]  
r1_nr_a[]  
time[]  
r2_a[]  
time[]  
r3_nr_a[]  
time[]  
r4_a[]  
time[]  
r5_a[]  
time[]
```

```
turnoff[]  
WAIT[398.02us]
```

```
r5_d[]  
time[]  
r4_d[]  
time[]  
r3_d[]
```

```
time[]
turnoff[]
time[]
turnoff[]
time[]
r2_l_a[]
time[]
turnoff[]
time[]
r4_l_a[]
time[]
turnoff[]
time[]
r2_d[]
time[]
r1_d[]
time[]
r0_d[]
time[]

turnoff[]
WAIT[397.99us]
turnoff[]
time[]
turnoff[]
time[]
r2_l_a[]
time[]
turnoff[]
time[]
r4_l_a[]
time[]
turnoff[]
time[]
turnoff[]
WAIT[3.99us]
turnoff[]
time[]
turnoff[]
time[]
r3_r_a[]
time[]
turnoff[]
time[]
r1_r_a[]
time[]
turnoff[]
time[]
turnoff[]
WAIT[397.99us]

r0_d[]
time[]
r1_d[]
```

```

time[]
r2_d[]
time[]
turnoff[]
time[]
turnoff[]
time[]
r3_r_a[]
time[]
turnoff[]
time[]
r1_r_a[]
time[]
turnoff[]
time[]
r3_d[]
time[]
r4_d[]
time[]
r5_d[]
time[]

turnoff[]
WAIT[398.02us]
r5_a[]
time[]
r4_n1_a[]
time[]
r3_a[]
time[]
r2_n1_a[]
time[]
r1_a[]
time[]
r0_a[]
time[]
turnoff[]
WAIT[34.99us]

turnoff[]
WAIT[5.99us]

WAIT[70us]

turnoff[]
E[397.968 us, 0.07 MHz]

# Readout data qubits

r5_Ad[]
time[]
r4_Ad[]
time[]
r3_Ad[]

```

```
time[]  
turnoff[]  
WAIT[34.99us]  
r2_Ad[]  
time[]  
r1_Ad[]  
time[]  
r0_Ad[]  
time[]
```

```
turnoff[]  
WAIT[8us]
```

```
END_COMMAND[]
```

## Rydberg AWG command string

The command string, used to program the amplitude, frequency, and phase for the 420-nm AOM for entangling gates and local SLM AOM for local detunings, is given below. Gate profiles (amplitude, detuning, and phase) are loaded from saved calibration files.

```
Wait[500.91 us]
```

```
### Start of circuit
```

```
# Start first QEC round
```

```
Pulse[420Amp[amplitudeFromFile,idx=1001,loops=1,delay=0.2],  
420Freq[detuningFromFile,idx=1001],  
420Phase[phaseFromFile,idx=1001, loops=1,delay=0.2],  
localShiftAmp[RabiPulseLoop,time=0.40,loops=1,A=1,delay = 0.18],  
localShiftFreq[fixedFrequency,detuning = 0.0]]  
Wait[467.800 us]  
Pulse[420Amp[amplitudeFromFile,idx=1001,loops=1,delay=0.2],  
420Freq[detuningFromFile,idx=1001],  
420Phase[phaseFromFile,idx=1001, loops=1,delay=0.2],  
localShiftAmp[RabiPulseLoop,time=0.40,loops=1,A=1,delay = 0.18],  
localShiftFreq[fixedFrequency,detuning = 0.0]]
```

```
Wait[467.800 us]
```

```
Pulse[420Amp[amplitudeFromFile,idx=1001,loops=1,delay=0.2],  
420Freq[detuningFromFile,idx=1001],  
420Phase[phaseFromFile,idx=1001, loops=1,delay=0.2],  
localShiftAmp[RabiPulseLoop,time=0.40,loops=1,A=1,delay = 0.18],  
localShiftFreq[fixedFrequency,detuning = 0.0]]
```

```
Wait[467.800 us]
```

```
Pulse[420Amp[amplitudeFromFile,idx=1001,loops=1,delay=0.2],  
420Freq[detuningFromFile,idx=1001],  
420Phase[phaseFromFile,idx=1001, loops=1,delay=0.2],  
localShiftAmp[RabiPulseLoop,time=0.40,loops=1,A=1,delay = 0.18],  
localShiftFreq[fixedFrequency,detuning = 0.0]]
```

```
Wait[467.800 us]
```

```
Wait[2570.02 us]
```

```
# Start second QEC round
```

```
Pulse[420Amp[amplitudeFromFile,idx=1001,loops=1,delay=0.2],  
420Freq[detuningFromFile,idx=1001],  
420Phase[phaseFromFile,idx=1001, loops=1,delay=0.2],  
localShiftAmp[RabiPulseLoop,time=0.40,loops=1,A=1,delay = 0.18],  
localShiftFreq[fixedFrequency,detuning = 0.0]]
```

Wait[467.800 us]

```
Pulse[420Amp[amplitudeFromFile,idx=1001,loops=1,delay=0.2],
420Freq[detuningFromFile,idx=1001],
420Phase[phaseFromFile,idx=1001, loops=1,delay=0.2],
localShiftAmp[RabiPulseLoop,time=0.40,loops=1,A=1,delay = 0.18],
localShiftFreq[fixedFrequency,detuning = 0.0]]
```

Wait[467.800 us]

```
Pulse[420Amp[amplitudeFromFile,idx=1001,loops=1,delay=0.2],
420Freq[detuningFromFile,idx=1001],
420Phase[phaseFromFile,idx=1001, loops=1,delay=0.2],
localShiftAmp[RabiPulseLoop,time=0.40,loops=1,A=1,delay = 0.18],
localShiftFreq[fixedFrequency,detuning = 0.0]]
```

Wait[467.800 us]

```
Pulse[420Amp[amplitudeFromFile,idx=1001,loops=1,delay=0.2],
420Freq[detuningFromFile,idx=1001],
420Phase[phaseFromFile,idx=1001, loops=1,delay=0.2],
localShiftAmp[RabiPulseLoop,time=0.40,loops=1,A=1,delay = 0.18],
localShiftFreq[fixedFrequency,detuning = 0.0]]
```

Wait[467.800 us]

Wait[2570.02 us]

# Start third QEC round

```
Pulse[420Amp[amplitudeFromFile,idx=1001,loops=1,delay=0.2],
420Freq[detuningFromFile,idx=1001],
420Phase[phaseFromFile,idx=1001, loops=1,delay=0.2],
localShiftAmp[RabiPulseLoop,time=0.40,loops=1,A=1,delay = 0.18],
localShiftFreq[fixedFrequency,detuning = 0.0]]
```

Wait[467.800 us]

```
Pulse[420Amp[amplitudeFromFile,idx=1001,loops=1,delay=0.2],
420Freq[detuningFromFile,idx=1001],
420Phase[phaseFromFile,idx=1001, loops=1,delay=0.2],
localShiftAmp[RabiPulseLoop,time=0.40,loops=1,A=1,delay = 0.18],
localShiftFreq[fixedFrequency,detuning = 0.0]]
```

Wait[467.800 us]

```
Pulse[420Amp[amplitudeFromFile,idx=1001,loops=1,delay=0.2],
420Freq[detuningFromFile,idx=1001],
420Phase[phaseFromFile,idx=1001, loops=1,delay=0.2],
localShiftAmp[RabiPulseLoop,time=0.40,loops=1,A=1,delay = 0.18],
localShiftFreq[fixedFrequency,detuning = 0.0]]
```



Wait[467.800 us]

Pulse[420Amp[amplitudeFromFile,idx=1001,loops=1,delay=0.2],  
420Freq[detuningFromFile,idx=1001],  
420Phase[phaseFromFile,idx=1001, loops=1,delay=0.2],  
localShiftAmp[RabiPulseLoop,time=0.40,loops=1,A=1,delay = 0.18],  
localShiftFreq[fixedFrequency,detuning = 0.0]]

Wait[467.800 us]

Wait[2570.02 us]

# Start fourth QEC round

Pulse[420Amp[amplitudeFromFile,idx=1001,loops=1,delay=0.2],  
420Freq[detuningFromFile,idx=1001],  
420Phase[phaseFromFile,idx=1001, loops=1,delay=0.2],  
localShiftAmp[RabiPulseLoop,time=0.40,loops=1,A=1,delay = 0.18],  
localShiftFreq[fixedFrequency,detuning = 0.0]]

Wait[467.800 us]

Pulse[420Amp[amplitudeFromFile,idx=1001,loops=1,delay=0.2],  
420Freq[detuningFromFile,idx=1001],  
420Phase[phaseFromFile,idx=1001, loops=1,delay=0.2],  
localShiftAmp[RabiPulseLoop,time=0.40,loops=1,A=1,delay = 0.18],  
localShiftFreq[fixedFrequency,detuning = 0.0]]

Wait[467.800 us]

Pulse[420Amp[amplitudeFromFile,idx=1001,loops=1,delay=0.2],  
420Freq[detuningFromFile,idx=1001],  
420Phase[phaseFromFile,idx=1001, loops=1,delay=0.2],  
localShiftAmp[RabiPulseLoop,time=0.40,loops=1,A=1,delay = 0.18],  
localShiftFreq[fixedFrequency,detuning = 0.0]]

Wait[467.800 us]

Pulse[420Amp[amplitudeFromFile,idx=1001,loops=1,delay=0.2],  
420Freq[detuningFromFile,idx=1001],  
420Phase[phaseFromFile,idx=1001, loops=1,delay=0.2],  
localShiftAmp[RabiPulseLoop,time=0.40,loops=1,A=1,delay = 0.18],  
localShiftFreq[fixedFrequency,detuning = 0.0]]

Wait[467.800 us]
