# Supplementary material for: Architectural mechanisms of a universal fault-tolerant quantum computer
Source: arXiv:2506.20661 ancillary file (2025-06-25)
Supplement: Supplementary file 2 [file RawExperimentalCommands_TesseractSpaceTime.pdf]

## Moving AWG command string

The command string used to program the RF waveforms for the Moving AWG, which control the positions and powers of moveable AOD tweezers, is given below. Waveforms are uploaded to different segments of the AWG using the SEGMENT[] command, which can then be individually looped or triggered with an external trigger.

Each move is defined using a MOVEAOD command. The initial position and power is specified for the first command when tweezers are turned on. For subsequent commands, the arguments specify where to move to (and optionally the power to ramp to), and take the form MOVEAOD[[x\_positions, y\_positions],[xpowers,ypowers],(time\_for\_move)]. Additional arguments such as SHIFT apply a global (x,y) coordinate shift to the coordinates in that move. Coordinates are given in 'SLM units' where 1 SLM unit here is approximately 5.6um in the x direction and 4.3um in the y direction.

### Define coordinates and powers

```
VAR[RESET[], MoveAOD[Initial[[-2],[-2]], InitialPows[[0.0001], [0.0001]],  
FinalPows[[0.0001], [0.0001]], 1 us]]
```

```
COMB[xe, [-0.02, 2.0, 16]]  
COMB[ye, [22.04, 2.0, 8]]
```

```
COMB[x1_e_alt, [-0.02, 4, 8]]  
VAR[x2_e_alt, [-0.02, 1.98, 7.98, 9.98, 15.98, 17.98, 23.98, 25.98]]  
COMB[y1_e_alt, [22.04, 4, 4]]  
VAR[y2_e_alt, [22.06, 24.06, 30.06, 32.06]]  
COMB[y_e_top, [22.06, 2, 4]]
```

```
COMB[x_store_SLM, [0.03, 2, 16]]  
COMB[y_st, [48, 1, 8]]
```

```
COMB[y_SSR, [4, 2, 8]]  
COMB[x_SSR, [0, 1, 32]]  
COMB[y2_SSR, [12, 2, 4]]
```

```
REPEAT_VAL[x_clear_pow, [0.271, 16]]  
REPEAT_VAL[y_clear_pow, [1.05, 8]]
```

```
REPEAT_VAL[x_image_pow, [0.2, 16]]  
REPEAT_VAL[y_image_pow, [0.4, 8]]
```

```
VAR[xSSR_32pow, [0.195, 0.195, 0.195, 0.195, 0.195, 0.195, 0.195, 0.190, 0.190,  
0.190, 0.190, 0.185, 0.185, 0.185, 0.185, 0.175, 0.175, 0.175, 0.175, 0.175,  
0.175, 0.175, 0.175, 0.170,0.170, 0.170,0.170, 0.170,0.165, 0.165,0.165,  
0.165]]
```

```
REPEAT_VAL[x0_32pow, [0.0, 32]]  
REPEAT_VAL[x0_pow, [0.0, 16]]  
REPEAT_VAL[x_init_8pow, [0.0, 8]]  
REPEAT_VAL[x_pickup_pow, [0.221, 16]]  
REPEAT_VAL[x_high_pow, [0.31, 16]]  
REPEAT_VAL[x2_high_pow, [0.39, 16]]  
REPEAT_VAL[x_high_8pow, [0.185, 8]]
```

```
REPEAT_VAL[x_gate_pow, [0.23, 16]]
```

```
REPEAT_VAL[x_gate_8pow, [0.095, 8]]
```

```
REPEAT_VAL[y0_pow, [0.0, 8]]
REPEAT_VAL[y0_4pow, [0.0, 4]]
VAR[y1_up_pow, [0.00001, 0.00002, 0.00003, 0.00004, 1.05, 1.05, 1.05, 1.05]]
REPEAT_VAL[y2_up_pow, [0.93, 8]]
VAR[y3_up_pow, [1.15, 1.12, 1.09, 1.05, 0.97, 0.93, 0.93, 0.93]]
REPEAT_VAL[y_4pow, [0.6, 4]]
VAR[y2_high_4pow, [0.98, 0.98, 0.98, 0.98]]
REPEAT_VAL[y_high_pow, [1.05, 8]]
VAR[ySSR_4pow, [1.50, 1.45, 1.35, 1.30]]
REPEAT_VAL[y_lowSSR_4pow, [1.21, 4]]
```

### First segment, used to clear unwanted atoms from entangling zone traps

```
SEGMENT[1, LOOP_UNTIL_TRIG]
MoveAOD[Initial[xe, ye],
InitialPows[x0_pow, y0_pow],
FinalPows[x_clear_pow, y_clear_pow], 0.05 ms]
MoveAOD[[xe, ye], SHIFT[-1, -1], 0.05 ms]
MoveAOD[Initial[x_store_SLM, y_st],
InitialPows[x0_pow, y0_pow],
FinalPows[x_clear_pow, y_clear_pow], 0.05 ms]
MoveAOD[[x_store_SLM, y_st], SHIFT[-1, -1], 0.05 ms]
WAIT[0.01 ms]
```

```
SEGMENT[2]
WAIT[214 us]
RESET[]
```

### Move atoms to their positions for the start of the circuit

```
SEGMENT[4]
WAIT[10 us]
MoveAOD[Initial[xe, y_SSR],
InitialPows[x0_pow, y0_pow],
FinalPows[x_high_pow, y1_up_pow], SHIFT[0, 0], YPHASES[6.2401, 2.1642, 3.1614,
4.1102, 3.6525, 5.2447, 3.1304, 1.1961], 0.15 ms]
MoveAOD[[xe, y_SSR], SHIFT[0.5, 0], 0.1 ms]
MoveAOD[[xe, y_SSR], SHIFT[0.5, 8], 0.3 ms]
MoveAOD[[xe, y_SSR], SHIFT[1, 8], 0.1 ms]
MoveAOD[[xe, y_SSR], FinalPows[x_high_pow, y2_up_pow], SHIFT[1, 8], 0.15 ms]
MoveAOD[[xe, y_SSR], SHIFT[0.5, 8], 0.1 ms]
MoveAOD[[xe, y_st], SHIFT[0.5, 0.0], 0.4 ms]
MoveAOD[[xe, y_st], SHIFT[0.0, 0.0], 0.1 ms]
MoveAOD[[xe, y_st], FinalPows[x0_pow, y0_pow], SHIFT[0.0, 0.0], 0.15 ms]
NOTE[Group A in storage zone]
```

```
SAVE_PREVIOUS[]
SAVE_PREVIOUS[]
```

```
WAIT[642.5 us]
```

RESET[]

### Start circuit here (looping single waveform per layer)

SEGMENT[5, LOOP\_UNTIL\_TRIG]

WAIT[4 us]

RESET[]

NOTE[Group B: Readout to entangling]

MoveAOD[Initial[xe, y\_SSR],

InitialPows[x0\_pow, y0\_pow],

FinalPows[x\_high\_pow, y1\_up\_pow], SHIFT[0, 1], YPHASES[6.2401, 2.1642, 3.1614, 4.1102, 3.6525, 5.2447, 3.1304, 1.1961], 0.15 ms]

MoveAOD[[xe, y\_SSR], SHIFT[0.5, 1], 0.1 ms]

MoveAOD[[xe, y\_SSR], SHIFT[0.5, 9], 0.25 ms]

MoveAOD[[xe, y\_SSR], SHIFT[1, 9], 0.1 ms]

MoveAOD[[xe, y\_SSR], FinalPows[x\_high\_pow, y2\_up\_pow], SHIFT[1, 9], 0.15 ms]

MoveAOD[[xe, y\_SSR], SHIFT[0.5, 9], 0.1 ms]

MoveAOD[[xe, ye], SHIFT[0.5, 0], 0.25 ms]

MoveAOD[[xe, ye], SHIFT[0, 0], 0.1 ms]

MoveAOD[[xe, ye], FinalPows[x0\_pow, y0\_pow], SHIFT[0,0], 0.15 ms]

NOTE[Group B prep]

WAIT[100 us]

NOTE[First gate layer of state prep]

MoveAOD[Initial[x1\_e\_alt, ye],

InitialPows[x\_init\_8pow, y0\_pow],

FinalPows[x\_high\_8pow, y\_high\_pow], SHIFT[2, 0], 0.15 ms]

MoveAOD[[x1\_e\_alt, ye], SHIFT[2, 0.5], 0.1 ms]

MoveAOD[[x1\_e\_alt, ye], SHIFT[0.3, 0.5], 0.25 ms]

MoveAOD[[x1\_e\_alt, ye], SHIFT[0.3, 0.5], FinalPows[x\_gate\_8pow, y\_high\_pow], 0.05 ms]

MoveAOD[[x1\_e\_alt, ye], SHIFT[0.3, 0], 0.095 ms]

WAIT[10 us]

MoveAOD[[x1\_e\_alt, ye], SHIFT[0.3, 0.5], 0.095 ms]

MoveAOD[[x1\_e\_alt, ye], SHIFT[0.3, 0.5], FinalPows[x\_high\_8pow, y\_high\_pow], 0.05 ms]

MoveAOD[[x1\_e\_alt, ye], SHIFT[2, 0.5], 0.25 ms]

MoveAOD[[x1\_e\_alt, ye], SHIFT[2, 0], 0.1 ms]

MoveAOD[[x1\_e\_alt, ye], FinalPows[x\_init\_8pow, y0\_pow], SHIFT[2, 0], 0.15 ms]

WAIT[99 us]

RESET[]

NOTE[Second gate layer of state prep]

MoveAOD[Initial[xe, y1\_e\_alt],

InitialPows[x0\_pow, y0\_4pow],

FinalPows[x\_high\_pow, y\_4pow], SHIFT[0, 0], 0.15 ms]

MoveAOD[[xe, y1\_e\_alt], SHIFT[0.5, 0], 0.1 ms]

```

MoveAOD[[xe, y1_e_alt], SHIFT[0.5, 2], 0.25 ms]
MoveAOD[[xe, y1_e_alt], SHIFT[0.5, 2], FinalPows[x_gate_pow, y_4pow], 0.05 ms]
MoveAOD[[xe, y1_e_alt], SHIFT[0.3, 2], 0.095 ms]
WAIT[10 us]
MoveAOD[[xe, y1_e_alt], SHIFT[0.5, 2], 0.095 ms]
MoveAOD[[xe, y1_e_alt], SHIFT[0.5, 2], FinalPows[x_high_pow, y_4pow], 0.05 ms]
MoveAOD[[xe, y1_e_alt], SHIFT[0.5, 0], 0.25 ms]
MoveAOD[[xe, y1_e_alt], SHIFT[0, 0], 0.1 ms]
MoveAOD[[xe, y1_e_alt], FinalPows[x0_pow, y0_4pow], SHIFT[0, 0], 0.15 ms]

WAIT[99 us]
RESET[]

```

```

NOTE[Third gate layer of state prep]
MoveAOD[Initial[x2_e_alt, ye],
InitialPows[x_init_8pow, y0_pow],
FinalPows[x_high_8pow, y_high_pow], SHIFT[4, 0], 0.12 ms]
MoveAOD[[x2_e_alt, ye], SHIFT[4, 0.5], 0.1 ms]
MoveAOD[[x2_e_alt, ye], SHIFT[0.3, 0.5], 0.3 ms]
MoveAOD[[x2_e_alt, ye], SHIFT[0.3, 0.5], FinalPows[x_gate_8pow, y_high_pow],
0.03 ms]
MoveAOD[[x2_e_alt, ye], SHIFT[0.3, 0], 0.095 ms]
WAIT[10 us]
MoveAOD[[x2_e_alt, ye], SHIFT[0.3, 0.5], 0.095 ms]
MoveAOD[[x2_e_alt, ye], SHIFT[0.3, 0.5], FinalPows[x_high_8pow, y_high_pow],
0.03 ms]
MoveAOD[[x2_e_alt, ye], SHIFT[4, 0.5], 0.3 ms]
MoveAOD[[x2_e_alt, ye], SHIFT[4, 0], 0.1 ms]
MoveAOD[[x2_e_alt, ye], FinalPows[x_init_8pow, y0_pow], SHIFT[4, 0], 0.12 ms]

WAIT[99 us]
RESET[]

```

```

NOTE[Fourth gate layer of state prep]
MoveAOD[Initial[xe, y2_e_alt],
InitialPows[x0_pow, y0_4pow],
FinalPows[x_high_pow, y_4pow], SHIFT[0, 4], 0.15 ms]
MoveAOD[[xe, y2_e_alt], SHIFT[0.5, 4], 0.1 ms]
MoveAOD[[xe, y2_e_alt], SHIFT[0.5, 0], 0.25 ms]
MoveAOD[[xe, y2_e_alt], SHIFT[0.5, 0], FinalPows[x_gate_pow, y_4pow], 0.05 ms]
MoveAOD[[xe, y2_e_alt], SHIFT[0.3, 0], 0.095 ms]
WAIT[10 us]
MoveAOD[[xe, y2_e_alt], SHIFT[0.5, 0], 0.095 ms]
MoveAOD[[xe, y2_e_alt], SHIFT[0.5, 0], FinalPows[x_high_pow, y_4pow], 0.05 ms]
MoveAOD[[xe, y2_e_alt], SHIFT[0.5, 4], 0.25 ms]
MoveAOD[[xe, y2_e_alt], SHIFT[0, 4], 0.1 ms]
MoveAOD[[xe, y2_e_alt], FinalPows[x0_pow, y_4pow], SHIFT[0, 4], 0.15 ms]

WAIT[99 us]
RESET[]

```

```

NOTE[Transversal cluster state in space]
MoveAOD[Initial[xe, y_e_top],

```

```

InitialPows[x0_pow, y0_4pow],
FinalPows[x_high_pow, y_4pow], SHIFT[0, 8], 0.15 ms]
MoveAOD[[xe, y_e_top], SHIFT[-0.5, 8], 0.1 ms]
MoveAOD[[xe, y_e_top], SHIFT[-0.5, 0], 0.4 ms]
MoveAOD[[xe, y_e_top], SHIFT[-0.3, 0], 0.095 ms]

WAIT[10 us]

MoveAOD[[xe, y_e_top], FinalPows[x_high_pow, y_4pow], SHIFT[-0.5, 0], 0.095 ms]
MoveAOD[[xe, y_e_top], SHIFT[-0.5, 0.5], 0.1 ms]
MoveAOD[[xe, y_e_top], SHIFT[-7.5, 0.5], 0.45 ms]
MoveAOD[[xe, y_e_top], SHIFT[-7.5, 0.5], 0.1 ms]
MoveAOD[[xe, y_e_top], SHIFT[-7.7, 0], 0.095 ms]

WAIT[10 us]

MoveAOD[[xe, y_e_top], FinalPows[x_high_pow, y_4pow], SHIFT[-7.5, 0.5], 0.095
ms]
MoveAOD[[xe, y_e_top], SHIFT[-7.5, 0.5], 0.1 ms]
MoveAOD[[xe, y_e_top], SHIFT[-0.5, 0.5], 0.45 ms]
MoveAOD[[xe, y_e_top], SHIFT[-0.5, 0], 0.1 ms]
MoveAOD[[xe, y_e_top], SHIFT[-0.3, 0], 0.095 ms]

WAIT[10 us]

MoveAOD[[xe, y_e_top], FinalPows[x_high_pow, y_4pow], SHIFT[-0.5, 0], 0.095 ms]
MoveAOD[[xe, y_e_top], SHIFT[-0.5, 8], 0.4 ms]
MoveAOD[[xe, y_e_top], SHIFT[0, 8], 0.1 ms]
MoveAOD[[xe, y_e_top],
FinalPows[x0_pow, y0_4pow], SHIFT[0, 8], 0.149 ms]
RESET[]

NOTE[Group A: storage to entangling]
MoveAOD[Initial[xe, y_st],
InitialPows[x0_pow, y0_pow],
FinalPows[x_high_pow, y2_up_pow], SHIFT[0, 0], 0.15 ms]
MoveAOD[[xe, y_st], SHIFT[0.5, 0], 0.1 ms]
MoveAOD[[xe, ye], SHIFT[0.5, 1], 0.37 ms]
MoveAOD[[xe, ye], SHIFT[1, 1], 0.13 ms]

WAIT[100 us]
MoveAOD[[xe, ye], FinalPows[x_gate_pow, y2_up_pow], SHIFT[1, 1], 0.03 ms]
MoveAOD[[xe, ye], SHIFT[0.3, 0], 0.115 ms]
NOTE[Transversal CNOT for time direction of cluster state]
WAIT[10 us]
MoveAOD[[xe, ye], SHIFT[1, 1], 0.115 ms]
MoveAOD[[xe, ye], FinalPows[x_high_pow, y2_up_pow], SHIFT[1, 1], 0.03 ms]
WAIT[100 us]

NOTE[Group A: Entangling to readout]
MoveAOD[[xe, y_SSR], SHIFT[0.5, 9], 0.3 ms]
MoveAOD[[xe, y_SSR], SHIFT[1, 9], 0.1 ms]

```

```
MoveAOD[[xe, y_SSR], FinalPows[x_high_pow, y1_up_pow], SHIFT[1, 9], 0.15 ms]
MoveAOD[[xe, y_SSR], SHIFT[0.5, 9], 0.1 ms]
MoveAOD[[xe, y_SSR], SHIFT[0.5, 1], 0.2 ms]
MoveAOD[[xe, y_SSR], SHIFT[0, 1], 0.1 ms]
MoveAOD[[xe, y_SSR], FinalPows[x0_pow, y0_pow], SHIFT[0, 1], 0.149 ms]
```

```
RESET[]
```

```
NOTE[Group B: Entangling to storage]
```

```
MoveAOD[Initial[xe, ye],
InitialPows[x0_pow, y0_pow],
FinalPows[x_high_pow, y2_up_pow], 0.15 ms]
MoveAOD[[xe, ye], SHIFT[0.5, 0], 0.1 ms]
MoveAOD[[xe, y_st], SHIFT[0.5, 0], 0.4 ms]
MoveAOD[[xe, y_st], SHIFT[0, 0], 0.1 ms]
MoveAOD[[xe, y_st], FinalPows[x0_pow, y0_pow], SHIFT[0, 0], 0.15 ms]
```

```
WAIT[1.499 ms]
```

```
RESET[]
```

```
NOTE[Readout group A]
```

```
MoveAOD[Initial[x_SSR, y2_SSR],
InitialPows[x0_32pow, y0_4pow],
FinalPows[xSSR_32pow, ySSR_4pow], SHIFT[0, 1], 0.25 ms]
MoveAOD[[x_SSR, y2_SSR], SHIFT[0.5, 1], 0.5 ms]
MoveAOD[[x_SSR, y2_SSR], SHIFT[0.5, 0], 0.3 ms]
MoveAOD[[x_SSR, y2_SSR], SHIFT[0, 0], 0.2 ms]
MoveAOD[[x_SSR, y2_SSR],
FinalPows[x0_32pow, y0_4pow], SHIFT[0, 0], 0.25 ms]
```

```
SSR_SAVE_PREVIOUS[]
```

```
WAIT[10.5 ms]
```

```
RESET[]
```

```
WAIT[14 us]
```

```
NOTE[Recombine spin states to original tweezer positions]
```

```
MoveAOD[Initial[x_SSR, y2_SSR],
InitialPows[x0_32pow, y0_4pow],
FinalPows[xSSR_32pow, ySSR_4pow], SHIFT[0, 0], 0.5 ms]
MoveAOD[[x_SSR, y2_SSR], SHIFT[0.5, 0], 0.5 ms]
MoveAOD[[x_SSR, y2_SSR], FinalPows[xSSR_32pow, ylowSSR_4pow], SHIFT[0.5, 0],
0.3 ms]
MoveAOD[[x_SSR, y2_SSR], SHIFT[0.5, 1], 0.8 ms]
MoveAOD[[x_SSR, y2_SSR], SHIFT[0, 1], 0.8 ms]
MoveAOD[[x_SSR, y2_SSR],
FinalPows[x0_32pow, y0_4pow], SHIFT[0, 1], 0.499 ms]
```

```
RESET[]
```

```
WAIT[11.427133 ms]
```

```
END_COMMAND[]
```

## Raman AWG command string

The command string used to program the I/Q waveforms and AOM amplitudes for local and global Raman control is given below. The command specifies the parameters for each single-qubit gate, which is then converted into the appropriate waveforms to modulate the light intensity and microwave phase and frequency (defined relative to the resonance frequency).

For local gates, the pulses are optionally gated on and off by the Raman AOD command.

Examples of typical commands are

Z : global Z rotation, in units of  $2\pi$

E : wait time, idling at the specified frequency

SC1\_ECHO : global SCROFULOUS Y( $\pi$ ) pulse for dynamical decoupling, idling at the specified frequency

SC1\_H\_LOCAL : SCROFULOUS Y( $\pi/2$ ) local gaussian pulses

SC1\_PI\_ECHO : SCROFULOUS Y( $\pi$ ) local gaussian pulses

FIXEDPUMPINGLOOPEDTTL: global Raman-assisted optical pumping

FIXEDPUMPINGLOOPEDTTLMOD: local Raman-assisted optical pumping

### Define variables for repeated commands

STARTVAR[ADDLAYER]

SC1\_ECHO[1.356885 ms, 0.02 MHz]

PREP\_GATES

SPACE\_TRANSVERSAL\_GATE # 3  $\pi$

TIME\_TRANSVERSAL\_GATE

STORE\_AND\_READ # 3  $\pi$

READOUT\_ECHOES # 5  $\pi$

REINITIALISE # 1  $\pi$

ENDVAR

STARTVAR[SPACE\_TRANSVERSAL\_GATE]

SC1\_ECHO[1.5 ms, 0.02 MHz]

Z[0.205]

SC1\_ECHO[0.19992 ms, 0.02 MHz]

Z[0.205]

SC1\_ECHO[1.5 ms, 0.02 MHz]

ENDVAR

STARTVAR[PREP\_GATES]

Z[0.0]

SC1\_H\_LOCAL[0.01us, 0.928, 4, 46 us, 0.5, 8, 1]

Z[0]

SC1\_ECHO[1.40792 ms, 0.02 MHz]

Z[0.205]

SC1\_H\_LOCAL[0.01us, 0.928, 4, 46 us, 0.5, 8, 1]

Z[0]

SC1\_ECHO[1.29992 ms, 0.02 MHz]

Z[0.205]

SC1\_H\_LOCAL[0.01us, 0.928, 4, 46 us, 0.5, 8, 1]

Z[0]

SC1\_ECHO[1.40792 ms, 0.02 MHz]

```

Z[0.205]
SC1_H_LOCAL[0.01us, 0.928, 4, 46 us, 0.5, 8, 1]
Z[0]
SC1_ECHO[1.29992 ms, 0.02 MHz]
Z[0.205]
SC1_H_LOCAL[0.01us, 0.886, 4, 46 us, 0.5, 8, 1]
SC1_ECHO[8 us, 0.02 MHz]
SC1_PI_LOCAL[0.01us, 0.96, 4, 46 us, 0.5, 8, 1]

```

ENDVAR

```

STARTVAR[TIME_TRANSVERSAL_GATE]
NOTE[storage to entangling here]
SC1_ECHO[0.150 ms, 0.02 MHz]
SC1_ECHO[0.600 ms, 0.02 MHz]

```

```

SC1_ECHO[100 us, 0.02 MHz]
Z[0.00]
SC1_ECHO[299.92 us, 0.02 MHz]
Z[0.205]
SC1_ECHO[53.92 us, 0.02 MHz]
Z[0.785]
SC1_H_LOCAL_PHASES[0.01us, 0.928, 4, 46 us, 0.5+0.5+0.5+0.5+0.5+0.5+0.5+0.5,
8, 1]
Z[-0.785]
SC1_ECHO[8 us, 0.02 MHz]
SC1_H_LOCAL[0.01us, 0.928, 4, 46 us, 0.5, 8, 1]
ENDVAR

```

```

STARTVAR[TIME_TRANSVERSAL_NO_GATE]
NOTE[storage to entangling here]
SC1_ECHO[0.150 ms, 0.02 MHz]
SC1_ECHO[0.600 ms, 0.02 MHz]

```

```

SC1_ECHO[100 us, 0.02 MHz]
Z[0.00]
SC1_ECHO[299.92 us, 0.02 MHz]
Z[0.00]
SC1_ECHO[53.92 us, 0.02 MHz]
Z[0.785]
SC1_H_LOCAL_PHASES[0.01us, 0.928, 4, 46 us, 0.5+0.5+0.5+0.5+0.5+0.5+0.5+0.5, 8,
1]
Z[-0.785]
SC1_ECHO[8 us, 0.02 MHz]
SC1_H_LOCAL[0.01us, 0.928, 4, 46 us, 0.5, 8, 1]
ENDVAR

```

```

STARTVAR[STORE_AND_READ]
NOTE[entangling to readout]
SC1_ECHO[0.5234 ms, 0.02 MHz]
SC1_ECHO[0.5234 ms, 0.02 MHz]
NOTE[entangling to storage]

```



```
SC1_ECHO[0.750 ms , 0.02 MHz]
SC1_ECHO[0.150 ms, 0.02 MHz]
ENDVAR
```

```
STARTVAR[READOUT_ECHOES]
NOTE[Lattice pumping here]
SC1_ECHO[3.9903 ms, 0.02 MHz]
```

```
SC1_ECHO[3.33 ms, 0.02 MHz]
SC1_ECHO[3.33 ms, 0.02 MHz]
SC1_ECHO[3.34 ms, 0.02 MHz]
```

```
Z[0.5]
SC1_ECHO[3.299975 ms, 0.02 MHz]
```

```
SC1_ECHO[3.34 ms, 0.02 MHz]
SC1_ECHO[3.33 ms, 0.02 MHz]
SC1_ECHO[3.33 ms, 0.02 MHz]
```

```
SC1_ECHO[106 us, 0.02 MHz]
```

```
ENDVAR
```

```
STARTVAR[REINITIALISE]
FIXEDPUMPINGLOOPEDTTLMOD[0, 2.6 us, -12.55 MHz, 12.55 MHz, 1, 6, 46, 10 us,
0.1us, 1, 464.5 us, local]
SC1_ECHO[14.38 us, 0.02 MHz]
FIXEDPUMPINGLOOPEDTTLMOD[0, 2.6 us, -12.55 MHz, 12.55 MHz, 1, 6, 46, 10 us,
0.1us, 0, 464.5 us, local]
ENDVAR
```

```
NOTE[CIRCUIT STARTS HERE]
```

```
ADDSEGMENT[0]
FIXEDPUMPINGLOOPEDTTL[0, 2.66 us, -11.6 MHz, 11.6 MHz, 1, 4, 24, 10 us, 0.1us]
E[10.625005 ms, 5MHz]
```

```
ADDSEGMENT[1]
E[1.356885 ms, 5 MHz]
PREP_GATES
SPACE_TRANSVERSAL_GATE
TIME_TRANSVERSAL_NO_GATE
STORE_AND_READ # 3 pi
READOUT_ECHOES # 5 pi
REINITIALISE # 1 pi
ADDSEGMENT[2]
ADDLAYER
ADDSEGMENT[3]
ADDLAYER
ADDSEGMENT[4]
```

ADDLAYER  
ADDSEGMENT[5]  
ADDLAYER  
ADDSEGMENT[6]  
ADDLAYER  
ADDSEGMENT[7]  
ADDLAYER  
ADDSEGMENT[8]  
ADDLAYER  
ADDSEGMENT[9]  
ADDLAYER  
ADDSEGMENT[10]  
ADDLAYER  
ADDSEGMENT[11]  
ADDLAYER  
ADDSEGMENT[12]  
ADDLAYER  
ADDSEGMENT[13]  
ADDLAYER  
ADDSEGMENT[14]  
ADDLAYER  
ADDSEGMENT[15]  
ADDLAYER  
ADDSEGMENT[16]  
ADDLAYER  
ADDSEGMENT[17]  
ADDLAYER  
ADDSEGMENT[18]  
ADDLAYER  
ADDSEGMENT[19]  
ADDLAYER  
ADDSEGMENT[20]  
ADDLAYER  
ADDSEGMENT[21]  
ADDLAYER  
ADDSEGMENT[22]  
ADDLAYER  
ADDSEGMENT[23]  
ADDLAYER  
ADDSEGMENT[24]  
ADDLAYER  
ADDSEGMENT[25]  
ADDLAYER  
ADDSEGMENT[26]  
ADDLAYER  
ADDSEGMENT[27]  
ADDLAYER  
ADDSEGMENT[28]  
ADDLAYER  
  
END\_COMMAND[ ]

## Raman AOD AWG command string

The command string used to program the RF waveforms for the Raman AOD AWG, which controls the positions and powers of 2D grids of optical tweezers used for local single-qubit gates, is given below.

Positions and powers are separately calibrated and loaded from a saved file. Different pulse configurations are specified by variables, for example 'r\_0\_t\_0\_' corresponding to pulses on row 0 at time step 0 of this particular circuit.

```
FILE[qubit_reuse_variables_tesseract_+++++.txt]
VAR[turnoff[], MOVEAOD[Initial[[-3],[-3]],INITIALPOWS[[0],[0]],10ns]]
VAR[extra_gap[], WAIT[108 us]]
VAR[pi_gap[], WAIT[7.99 us]]
VAR[RMgate_gap[], WAIT[1299.98 us]]
VAR[pump_gap, WAIT[9.99us]]

SEGMENT[1, LOOP_UNTIL_TRIG]

WAIT[1.35343 ms]

LOOPPULSES[r_0_t_0_, r_1_t_0_, r_2_t_0_, r_3_t_0_, r_4_t_0_, r_5_t_0_,
r_6_t_0_, r_7_t_0_, 46us]
turnoff[]
extra_gap[]
RMgate_gap[]

LOOPPULSES[r_7_t_1_, r_6_t_1_, r_5_t_1_, r_4_t_1_, r_3_t_1_, r_2_t_1_,
r_1_t_1_, r_0_t_1_, 46us]
turnoff[]
RMgate_gap[]

LOOPPULSES[r_0_t_2_, r_1_t_2_, r_2_t_2_, r_3_t_2_, r_4_t_2_, r_5_t_2_,
r_6_t_2_, r_7_t_2_, 46us]
turnoff[]
extra_gap[]
RMgate_gap[]

LOOPPULSES[r_7_t_3_, r_6_t_3_, r_5_t_3_, r_4_t_3_, r_3_t_3_, r_2_t_3_,
r_1_t_3_, r_0_t_3_, 46us]
turnoff[]
RMgate_gap[]

LOOPPULSES[r_0_t_4_, r_1_t_4_, r_2_t_4_, r_3_t_4_, r_4_t_4_, r_5_t_4_,
r_6_t_4_, r_7_t_4_, 46us]
turnoff[]
pi_gap[]
WAIT[46us]
turnoff[]

WAIT[3.95 ms]

WAIT[46us]
```

```

turnoff[]
pi_gap[]
WAIT[46us]
turnoff[]

WAIT[300 us]

LOOPPULSES[empty, empty, empty, empty, empty, empty, empty, empty, 46us]
turnoff[]
pi_gap[]
LOOPPULSES[r_aod0, r_aod1, r_aod2, r_aod3, empty, empty, empty, empty, 46us]
turnoff[]

WAIT[29.39950 ms]

LOOPVARS[bright_even,pump_gap,bright_odd,pump_gap,23] # looped local pi pulses
for Raman-assisted optical pumping

MOVEAOD[Initial[[-3],[-3]],INITIALPOWS[[0],[0]],10ns]

WAIT[484.5 us]

WAIT[1.35343 ms]

LOOPPULSES[r_0_t_0_, r_1_t_0_, r_2_t_0_, r_3_t_0_, r_4_t_0_, r_5_t_0_,
r_6_t_0_, r_7_t_0_, 46us]
turnoff[]
extra_gap[]
RMgate_gap[]

LOOPPULSES[r_7_t_1_, r_6_t_1_, r_5_t_1_, r_4_t_1_, r_3_t_1_, r_2_t_1_,
r_1_t_1_, r_0_t_1_, 46us]
turnoff[]
RMgate_gap[]

LOOPPULSES[r_0_t_2_, r_1_t_2_, r_2_t_2_, r_3_t_2_, r_4_t_2_, r_5_t_2_,
r_6_t_2_, r_7_t_2_, 46us]
turnoff[]
extra_gap[]
RMgate_gap[]

LOOPPULSES[r_7_t_3_, r_6_t_3_, r_5_t_3_, r_4_t_3_, r_3_t_3_, r_2_t_3_,
r_1_t_3_, r_0_t_3_, 46us]
turnoff[]
RMgate_gap[]

LOOPPULSES[r_0_t_4_, r_1_t_4_, r_2_t_4_, r_3_t_4_, r_4_t_4_, r_5_t_4_,
r_6_t_4_, r_7_t_4_, 46us]
turnoff[]
pi_gap[]
WAIT[46us]
turnoff[]

```

```
WAIT[3.95 ms]
```

```
WAIT[46us]  
turnoff[]  
pi_gap[]  
WAIT[46us]  
turnoff[]
```

```
WAIT[300 us]
```

```
LOOPPULSES[empty, empty, empty, empty, empty, empty, empty, empty, 46us]  
turnoff[]  
pi_gap[]  
LOOPPULSES[empty, empty, empty, empty, r_aod4, r_aod5, r_aod6, r_aod7, 46us]  
turnoff[]
```

```
WAIT[29.39939 ms]
```

```
LOOPVARS[bright_even,pump_gap,bright_odd,pump_gap,23] # looped local pi pulses  
for Raman-assisted optical pumping
```

```
MOVEAOD[Initial[[-3],[-3]],INITIALPOWS[[0],[0]],10ns]
```

```
WAIT[484.5 us]
```

```
END_COMMAND[]
```

## Rydberg AWG command string

The command string used to program the AOM amplitude, frequency, and phase for the 420-nm laser for entangling gates is given below. Gate profiles (amplitude, detuning, and phase) are loaded from saved calibration files.

```
Wait[2079.90 us]
Pulse[420Amp[amplitudeFromFile,idx=1002,loops=1],
420Freq[detuningFromFile,idx=1002],
420Phase[phaseFromFile,idx=1002, loops=1]]
Wait[1.398 ms]
Pulse[420Amp[amplitudeFromFile,idx=1002,loops=1],
420Freq[detuningFromFile,idx=1002],
420Phase[phaseFromFile,idx=1002, loops=1]]
Wait[1.398 ms]
Pulse[420Amp[amplitudeFromFile,idx=1002,loops=1],
420Freq[detuningFromFile,idx=1002],
420Phase[phaseFromFile,idx=1002, loops=1]]
Wait[1.398 ms]
Pulse[420Amp[amplitudeFromFile,idx=1002,loops=1],
420Freq[detuningFromFile,idx=1002],
420Phase[phaseFromFile,idx=1002, loops=1]]
Wait[1.498 ms]

Pulse[420Amp[amplitudeFromFile,idx=1002,loops=1],
420Freq[detuningFromFile,idx=1002],
420Phase[phaseFromFile,idx=1002, loops=1]]
Wait[0.848 ms]
Pulse[420Amp[amplitudeFromFile,idx=1002,loops=1],
420Freq[detuningFromFile,idx=1002],
420Phase[phaseFromFile,idx=1002, loops=1]]

Wait[2.598 ms]
Pulse[420Amp[amplitudeFromFile,idx=1002,loops=1],
420Freq[detuningFromFile,idx=1002],
420Phase[phaseFromFile,idx=1002, loops=1]]

Wait[30.6146 ms]
```
